# Supplementary material for: Sparse Autoencoders Find Highly Interpretable Features in Language Models
Source: arXiv:2309.08600 source file (2023-10-04)
Supplement: Supplementary file 1 [file aidan_erased_feature_interp.tex]

\iffalse
%\subsection{Interpreting Intervened Features}

\label{appendix:concept-erasure-feature-interp}

We plot token activation histograms (see Section \ref{section:case_studies}) for the features we ablate in Section \ref{section:concept_erasure}. Note that pronoun-related tokens (such as `\_she', `\_her' etc) appear in the top-5 most commonly activated tokens for the first three layers' features.

\begin{figure}[h]
    \centering
    \includegraphics[width=0.5\textwidth]{images/aidan/hist_0_1486_0.50.png}
    \includegraphics[width=0.5\textwidth]{images/aidan/hist_1_309_0.50.png}
    \includegraphics[width=0.5\textwidth]{images/aidan/hist_2_1374_0.50.png}
    
    \includegraphics[width=0.5\textwidth]{images/aidan/hist_3_855_0.57.png}
    \includegraphics[width=0.5\textwidth]{images/aidan/hist_4_1249_0.54.png}
    \caption{Histograms of token activations for the ablated directions in Section \ref{section:concept_erasure}.}
\end{figure}
\fi

% \subsection{KL-Divergence on Training Distribution}

\label{appendix:kl_div_pile}

We measure the disruption to model behaviour by calculating the KL-divergence of the ablated model from the base model on the first 10,000 sequences from the Pile dataset \citep{gao2020pile}. We find that erasing the relevant dictionary features causes significantly less KL-divergence than difference-in-means projection or LEACE (Figure \ref{fig:kl-across-depth}).

\begin{figure}[h]
    \centering
    \includegraphics[width=0.8\textwidth]{images/aidan/kl_across_depth.png}
    \caption{KL-divergence of the ablated model from the base model on the Pile, versus the layer the concept erasure intervention is performed at. The last datapoint for the difference-in-means edit has been ommitted as it is multiple orders of magnitude larger than all other datapoints.}
    \label{fig:kl-across-depth}
\end{figure}

\iffalse

\subsection{Erasure on the Transfer Dataset}

While dictionary erasure methods do not always transfer to the secondary task, we find that the `correct' (most optimal) features for erasure are in the top-four best-performing features of the other dataset (Figure \ref{fig:transfer_optimum_perf}).

\fi

\iffalse
\subsection{Concept Erasure on Last Token}

\label{appendix:concept_erasure_last_position}

We perform the same concept erasure experiment as in Section \ref{section:concept_erasure}, restricting edits to the last token position and re-fitting the difference-in-means and LEACE projections (Figure \ref{fig:erasure_last_pos}). We note that here LEACE achieves perfect performance with minimal intervention, as our i.i.d. assumption is correct.

\begin{figure}[h]
    \centering
    \includegraphics[width=0.8\textwidth]{images/aidan/erasure_across_depth_last_pos.png}
    \caption{Erasure via editing the last token position of the gender-prediction prompt.}
    \label{fig:erasure_last_pos}
\end{figure}
\fi
