# Supplementary material for: Sparse Autoencoders Find Highly Interpretable Features in Language Models
Source: arXiv:2309.08600 source file (2023-10-04)
Supplement: Supplementary file 3 [file aidan_edit_mag.tex]

% \begin{figure}
%     \centering
%     \includegraphics[width=.8\textwidth]{images/aidan/feature_ident_curve_edit_l11.png}
%     \caption{We are able to steer the model to the same degree via patching as other decompositions at the same magnitude of intervention. We find that the magnitude of intervention versus steering amount Pareto frontier shifts to the left as the sparsity of the learned dictionary decomposition increases, albeit at the cost of a larger maximum steering amount.}
%     \label{fig:edit_mag_vs_steering}
% \end{figure}

% We found that as well as achieving steering in a smaller number of patches, we are also able to steer to a greater degree with a smaller edit (Figure \ref{fig:edit_mag_vs_steering}).
