# Supplementary material for: Sparse Autoencoders Find Highly Interpretable Features in Language Models
Source: arXiv:2309.08600 source file (2023-10-04)
Supplement: Supplementary file 4 [file aidan_number_of_features.tex]

% As of 8/15 we're NOT planning for this to not be in the 8/18 draft. Omit for now

Aidan's work, describing what we did to estimate the number of features, including any figures, etc.
