# Supplementary material for: Sparse Autoencoders Find Highly Interpretable Features in Language Models
Source: arXiv:2309.08600 source file (2023-10-04)
Supplement: Supplementary file 5 [file feature_MCS_results.tex]

can use MCS to look at the similarity of the dictionaries, between dicts of the same layer/same hparams, same layer/diff hparams, diff layer/same hparams
\begin{figure}
    \centering
    \includegraphics[width=0.8\textwidth]{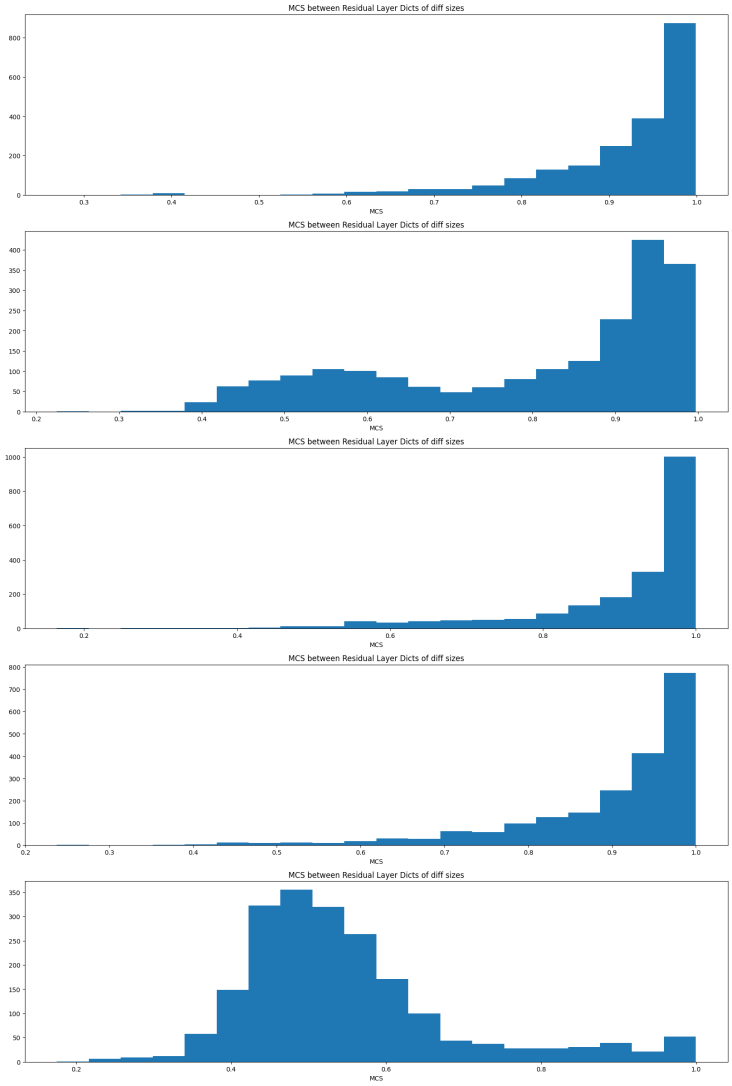}
    \caption{Graphs showing MCS results}
    \label{fig:mcs_place}
\end{figure}
