# Supplementary material for: Sparse Autoencoders Find Highly Interpretable Features in Language Models
Source: arXiv:2309.08600 source file (2023-10-04)
Supplement: Supplementary file 6 [file outlier_dimensions.tex]

Outlier dimensions are dimensions in the residual stream with extremely high values. For Pythia-70M, the top 3 dimensions have max-activating datapoints that are TODO standard deviations above the mean. They have caused problems when quantising language models \citep{dettmers2022llmint8}, and been studied before in a variety of models TODO cite
